# Supplementary material for: Predicting Methane Adsorption in Metal-Substituted MOFs: A Comparative Study between Density Functional Theory and Machine Learning
Source: arXiv:2504.15034 source file (2025-04-28)

# Supporting Information

# Predicting Methane Adsorption in Metal-Substituted MOFs: A Comparative Study between Density Functional Theory and Machine Learning

Karim Aljamal and Xiao Wang*

*Department of Chemistry and Biochemistry, University of California Santa Cruz, California 95064 USA*

*Corresponding author: Xiao Wang

## Contents

Table S1. Performance of fine-tuned PMTransformer models as a function of training dataset size.

Table S2. Structural changes upon metal substitution in the three MOFs studied in this work.

Figure S1. Training metrics of the HoA (heat of adsorption) model as a function of epochs.

Figure S2. Training metrics of the uptake (volumetric uptake) model as a function of epochs.

Figure S3. Structures of the four hypothetical MOFs randomly selected from the hMOF dataset.

**Table S1.** Performance of fine-tuned PMTransformer models as a function of training dataset size. The mean absolute error (MAE) and $R^2$ values are shown for the HoA (heat of adsorption) model and the uptake (volumetric uptake) model against the reference data from the hMOF dataset.

| | Heat of Adsorption | | Uptake | |
|---|---|---|---|---|
| Dataset size | MAE (kJ/mol) | $R^2$ | MAE ($cm^3/cm^3$) | $R^2$ |
| 1024 | 0.97 | 88.56% | 14.11 | 83.79% |
| 2048 | 0.90 | 89.06% | 11.36 | 84.39% |
| 4096 | 0.87 | 89.71% | 9.55 | 90.44% |
| 8192 | 0.79 | 92.56% | 8.52 | 91.93% |
| 32768 | 0.77 | 91.31% | 6.97 | 94.44% |

**Table S2.** Structural changes upon metal substitution in the three MOFs studied in this work. Unit cell volumes (in Å$^3$) and selected bond distances (in Å) for Cu and Zn variants of M-HKUST-1, M-ATC, and M-ZIF-8 are obtained after DFT optimization. Percentage changes in metal-substituted MOFs relative to original MOFs are shown in parentheses.

| Metal (M) | Cu | Zn |
|---|---|---|
| | **M-HKUST-1** | |
| Unit cell volume | 18557.73 | 19195.51 (3.4%) |
| M-M | 2.49 | 2.57 (3.2%) |
| M-O | 1.97 | 2.02 (2.5%) |
| M-$CH_4$ (site I) | 3.04 | 2.59 (-14.8%) |
| | **M-ATC** | |
| Unit cell volume | 1056.37 | 1088.60 (3.1%) |
| M-M (same paddlewheel) | 2.49 | 2.60 (4.4%) |
| M-M (opposing paddlewheels) | 6.03 | 6.04 (0.2%) |
| M-O | 1.97 | 2.02 (2.5%) |
| M-$CH_4$ (site I) | 3.01 | 3.00 (-0.3%) |
| | **M-ZIF-8** | |
| Unit Cell Volume | 4472.46 (-8.6%) | 4891.36 |
| M-N | 1.97 (-1.0%) | 1.99 |
| (C=C)-$CH_4$ (site I) | 3.55 (-1.9%) | 3.62 |

**Figure S1.** Training metrics of the HoA (heat of adsorption) model as a function of epochs. The mean absolute error (MAE) and mean squared error (MSE) values per epoch are shown against the reference data from the hMOF dataset.

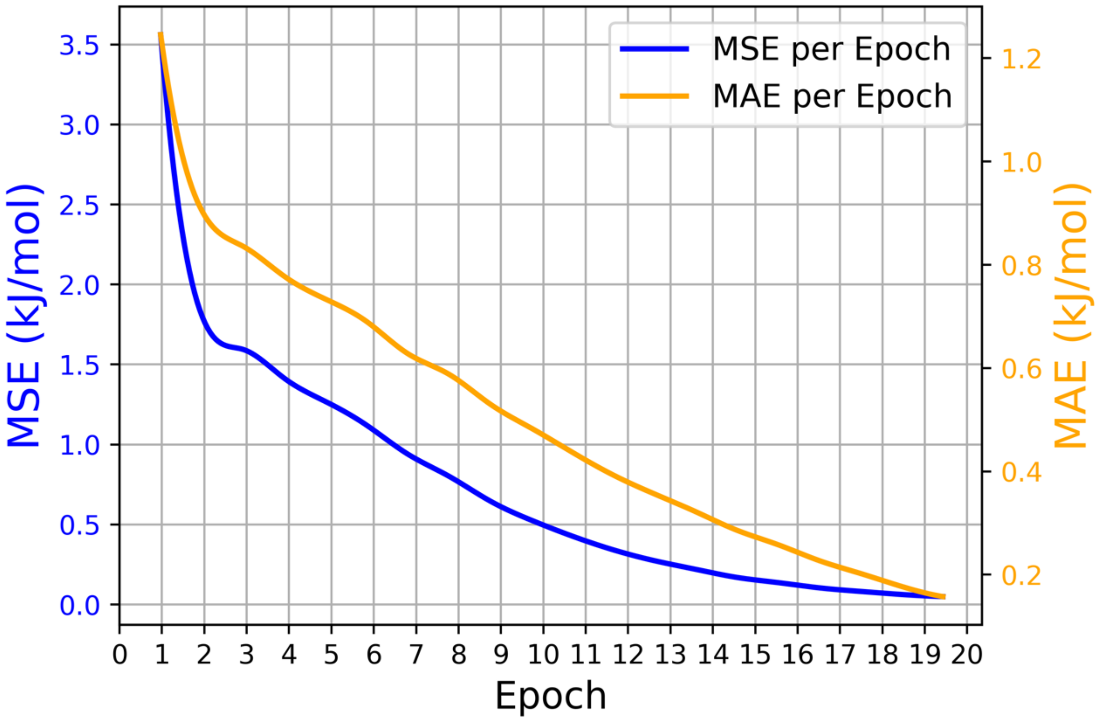

**Figure S2.** Training metrics of the uptake (volumetric uptake) model as a function of epochs. The mean absolute error (MAE) and mean squared error (MSE) values per epoch are shown against the reference data from the hMOF dataset.

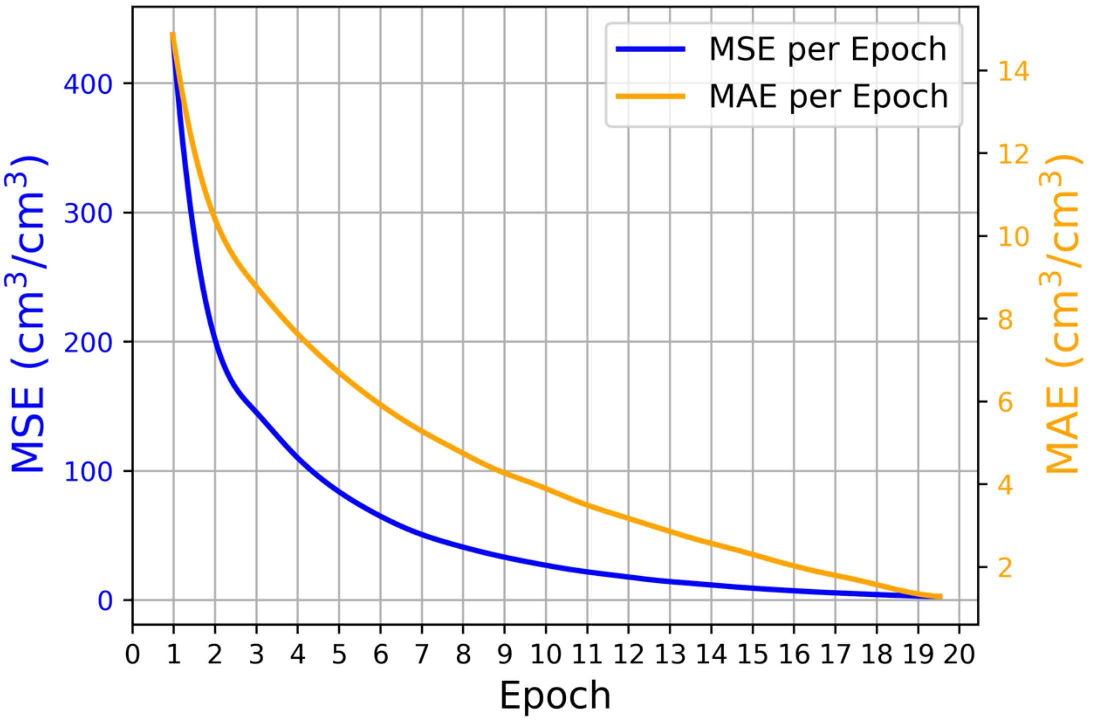

**Figure S3.** Structures of the four hypothetical MOFs randomly selected from the hMOF dataset. These MOFs are identified as (a) hMOF-32693, (b) hMOF-5041020, (c) hMOF-5052408, and (d) hMOF-5073729 in the database.

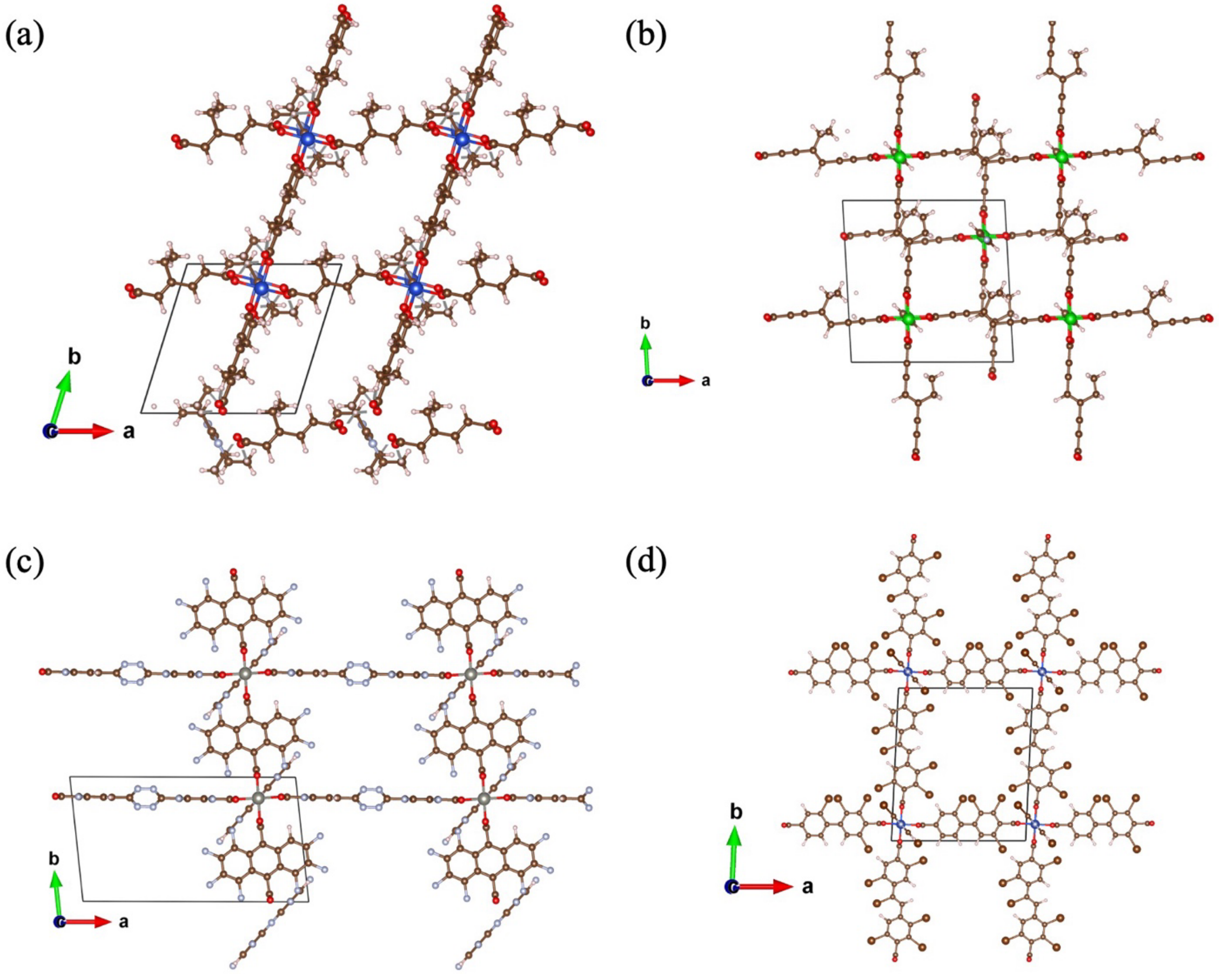

Supplement: Supplementary file 1 [file Supporting_Info.pdf]
